# Supplementary material for: Triple Junctions as Dislocation-Like Defects: The Role of Grain Boundary Crystallography Revealed by Experiment and Atomistic Simulation
Source: arXiv:2602.04530 ancillary file (2026-02-04)
Supplement: Supplementary file 1 [file supplemental-material.pdf]

## SUPPLEMENTAL MATERIAL

### Triple Junctions as Dislocation-Like Defects: The Role of Grain Boundary Crystallography Revealed by Experiment and Atomistic Simulation

Tobias Brink, Saba Saood, Peter Schweizer, Jörg Neugebauer, and Gerhard Dehm  
*Max Planck Institute for Sustainable Materials, Max-Planck-Straße 1, 40237 Düsseldorf, Germany*

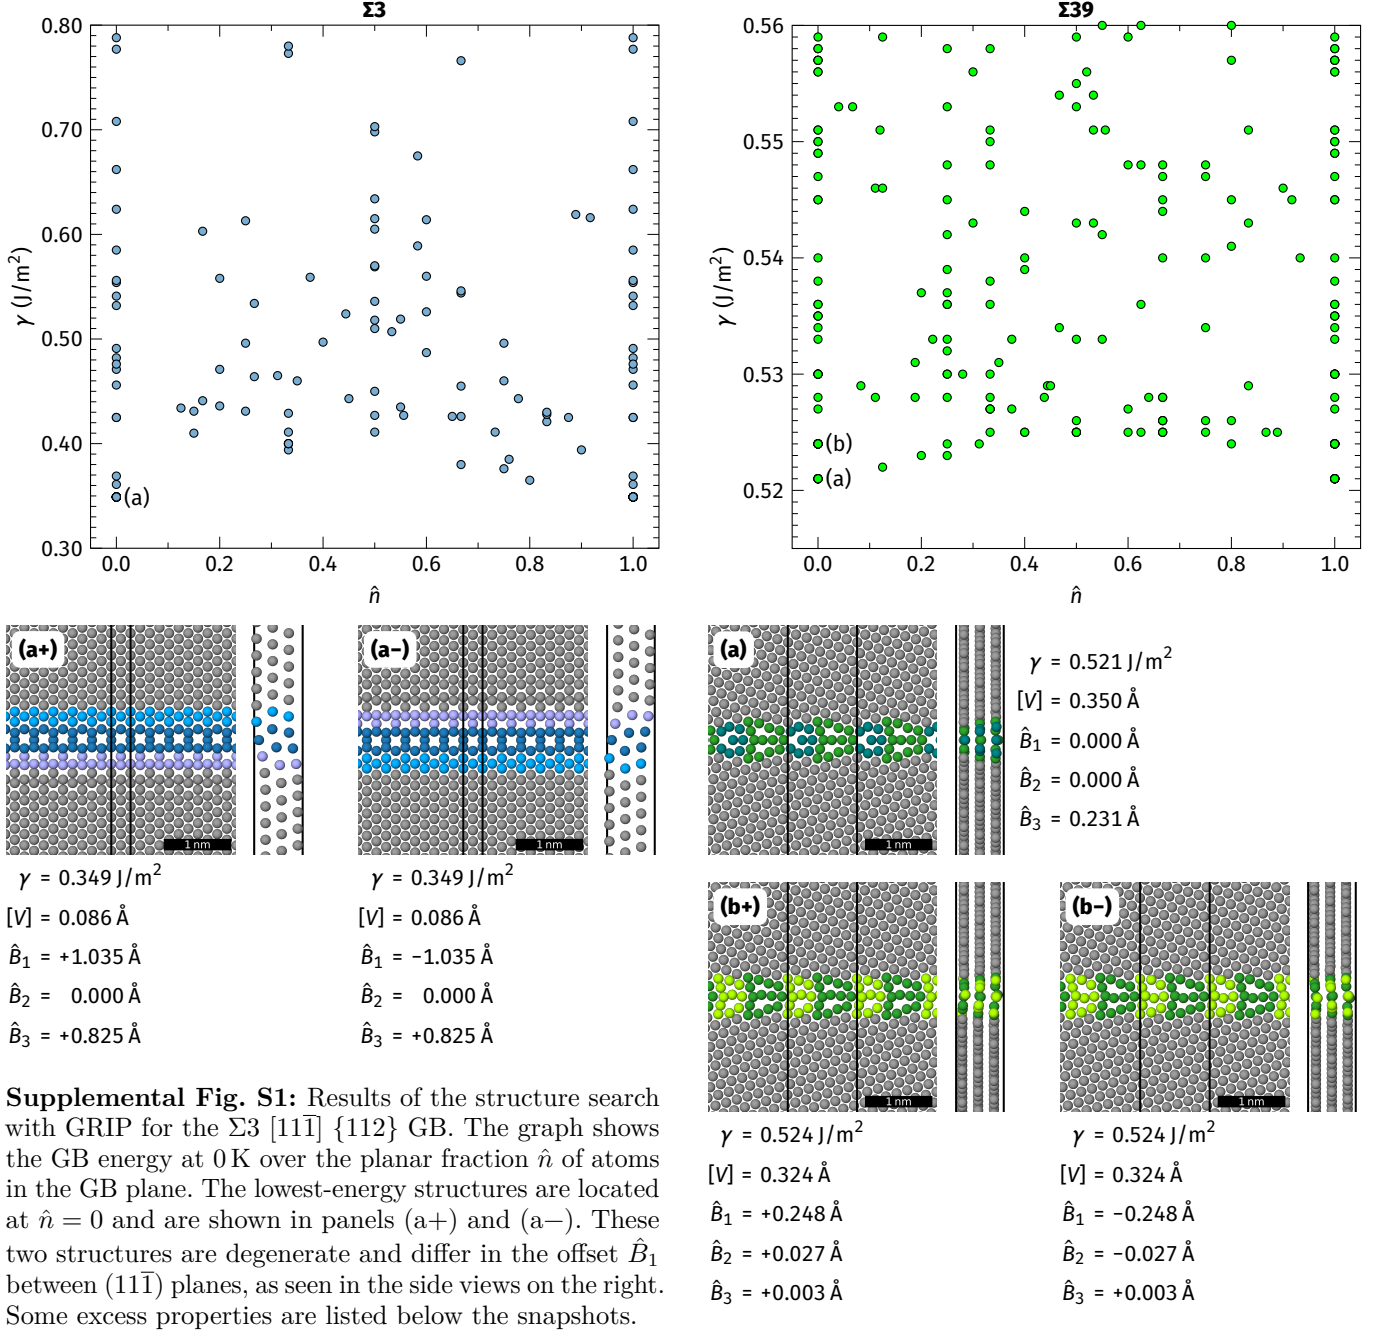

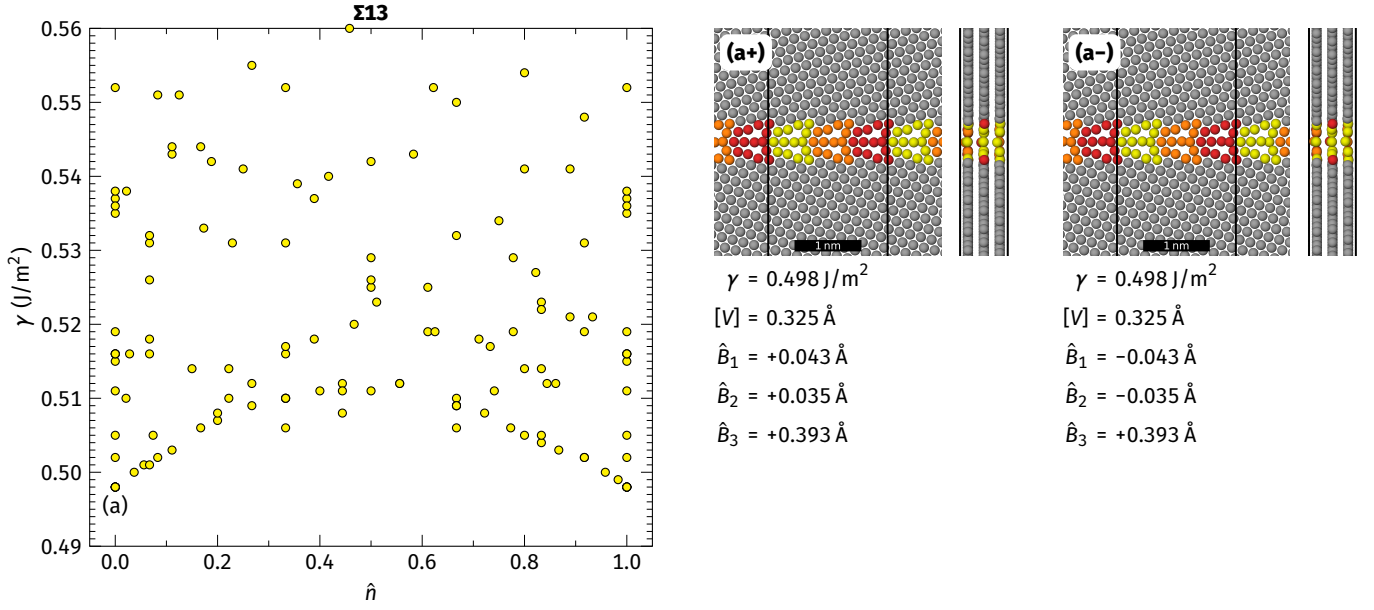

**Supplemental Fig. S3:** Results of the structure search with GRIP for the  $\Sigma 13$   $[11\bar{1}]$   $\{134\}$  GB. (a $\pm$ ) Two degenerate versions exist of the lowest energy structure. Like all GBs in this work, these also have a planar fraction of  $\hat{n} = 0$ .

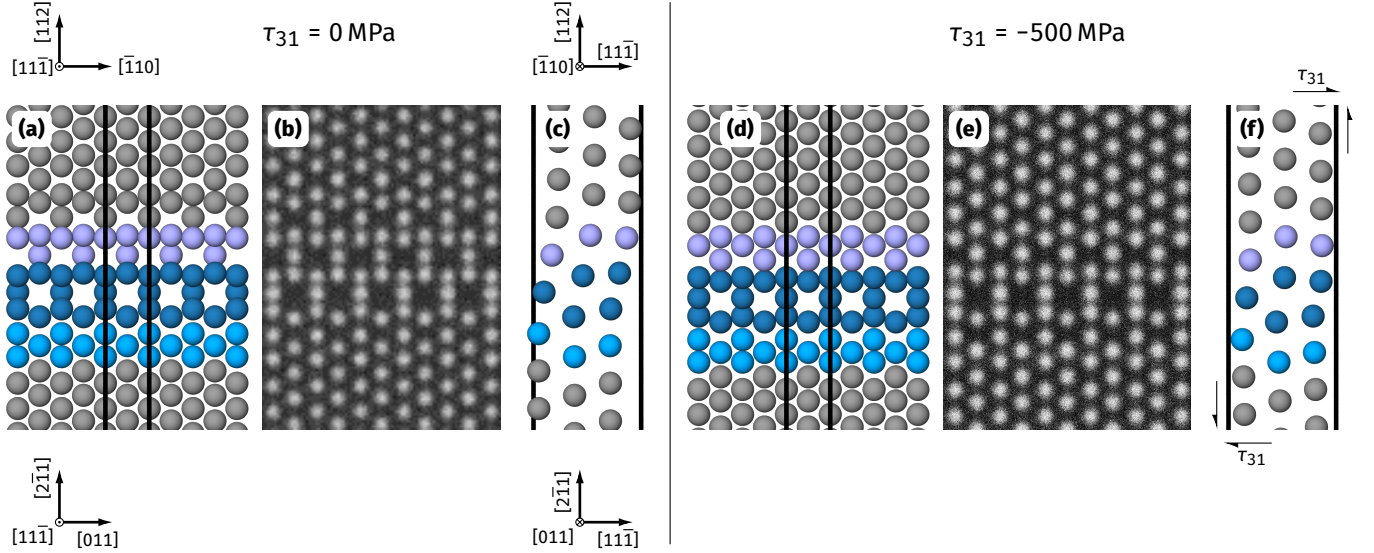

**Supplemental Fig. S4:** (a) The  $\Sigma 3$  GB as obtained with struture search (Supplemental Fig. S1). (b) A STEM image simulation of this structure does not fit well to the experimentally observed  $\Sigma 3$  GB. (c) The  $\Sigma 3$  GB has a large offset  $\hat{B}_1$  between  $(11\bar{1})$  planes compared to the  $\Sigma 39$  and  $\Sigma 13$  GBs. Thus, it is likely that the  $\Sigma 3$  GB is under stress near the triple junction, in particular the  $\tau_{31}$  component (f). (d) We thus applied such a stress and (e) repeated the STEM image simulation. The resulting image fits better to the experiment (Fig. 2 in the main text) and to the simulated GB near the triple junction (Fig. 5 in the main text).

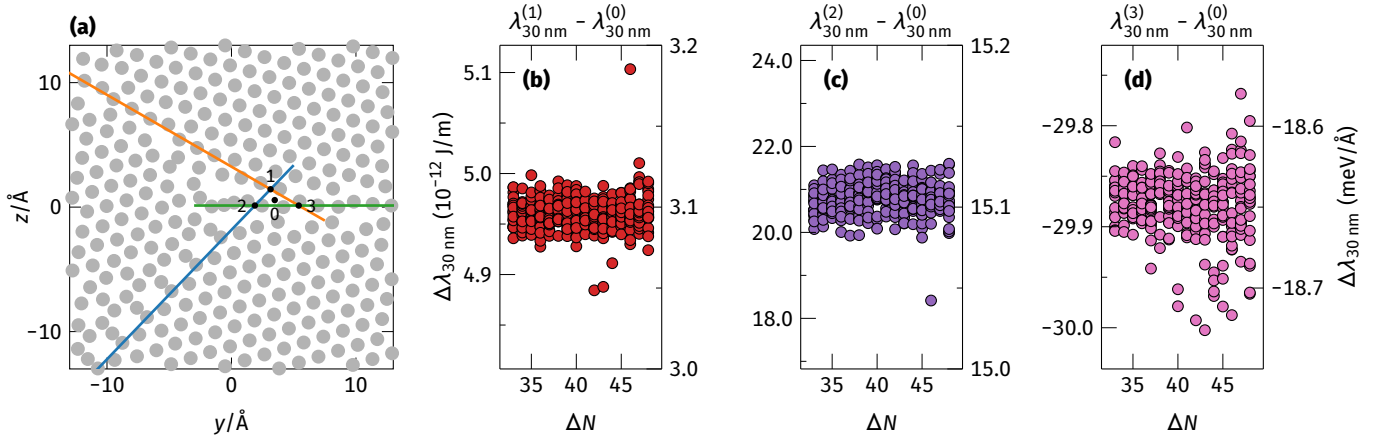

**Supplemental Fig. S5:** Influence of the choice of assumed triple junction center. (a) We define the junction center by drawing lines through the centers of the three GBs, leading to three intersection points 1,2,3. The average of these points is taken to be our center point 0 for the calculation of excess energies. We estimate the systematic error of our assumption by also calculating excess energies around center points 1, 2, and 3. (b)–(d) For all triple junction core structures from Fig. 6 in the main text, we calculate the difference between  $\lambda_{30 \text{ nm}}$  calculated with center point 0 and center point 1, 2, or 3. The resulting energy differences have very low scatter (note the units of the axes) and the error is thus systematic and not random. Consequently, the determination of the minimum energy triple junction core structure for a given Burgers vector is robust against the choice of center point. The comparison between structures with different Burgers vectors, however, is subject to this error.

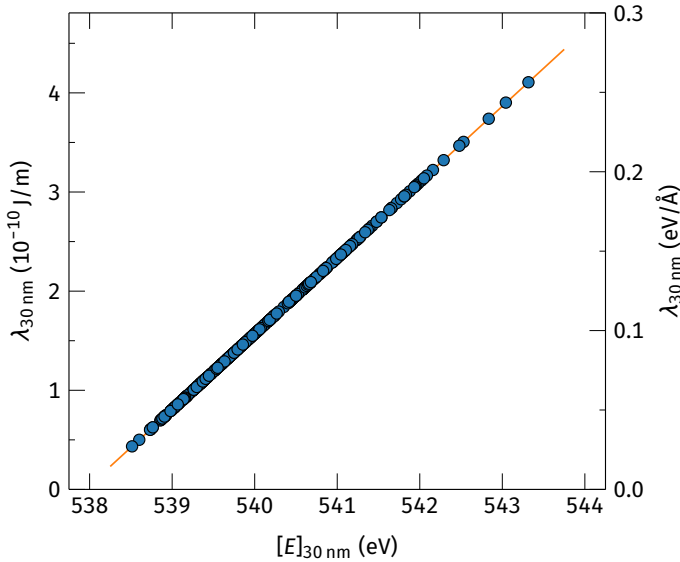

**Supplemental Fig. S6:** The excess energy  $[E]$  and the line energy  $\lambda$  are related via  $\lambda = ([E] - A \sum_i \gamma_i) / L_x$  (Eq. 8 in the main text). Thus, the energy change in  $[E]$  and  $\lambda$  due to a different junction core structure must be linearly related. Here, we show that this is exactly true for the example of the data from Fig. 6 in the main paper, with  $[E]$  and  $\lambda$  taken within a radius of 30 nm around the triple junction line. This means that either  $[E]_{30 \text{ nm}}$  or  $\lambda_{30 \text{ nm}}$  can serve as equivalent optimization criteria to find the most stable junction core structure for a given Burgers vector.

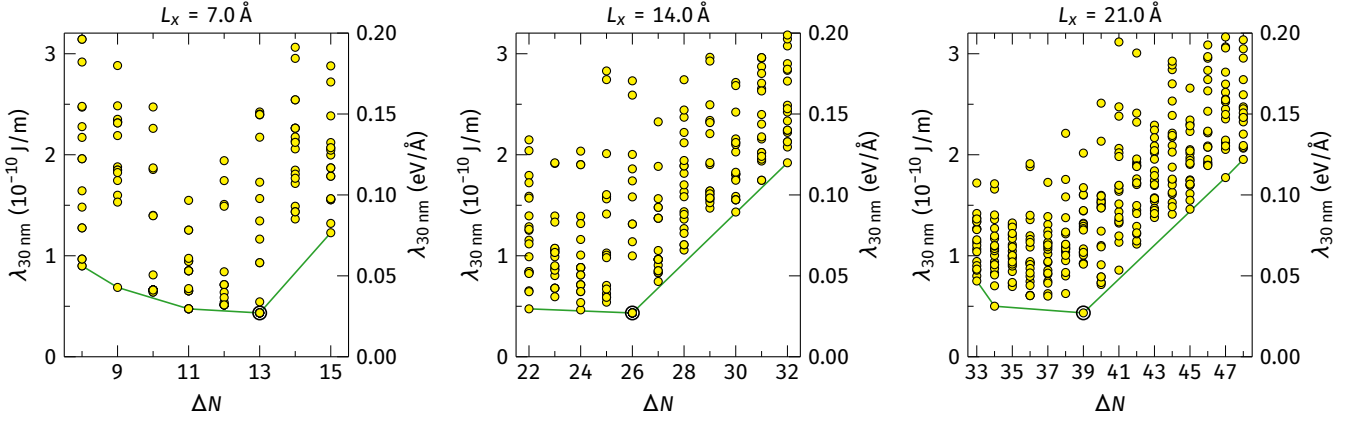

**Supplemental Fig. S7:** To reproduce the experimental triple junction, we performed structure searches with simulation boxes of different thickness. We used one, two, or three unit cells along the tilt axis direction ( $x$ ). The largest thickness corresponds to the results of Fig. 6 in the main text. We obtain the exact same minimum energy triple junction structure in all cases. Only the number of inserted atoms scales obviously with the thickness.

**Supplemental Table S-I:** CSL and DSC vectors for the three observed GBs. The vectors are expressed in terms of the crystal coordinate system of the relevant bottom crystal as indicated in Figs. 2–4 in the main text.

|                 | $\theta$       | $\mathbf{v}_{\text{CSL}}^{(1)}$ | $\mathbf{v}_{\text{CSL}}^{(2)}$ | $\mathbf{v}_{\text{CSL}}^{(3)}$                                  | $\mathbf{d}_{\text{SC}}^{(1)}$ | $\mathbf{d}_{\text{SC}}^{(2)}$ | $\mathbf{d}_{\text{SC}}^{(3)}$                                    |
|-----------------|----------------|---------------------------------|---------------------------------|------------------------------------------------------------------|--------------------------------|--------------------------------|-------------------------------------------------------------------|
| $\Sigma 3$      | $60.000^\circ$ | $a/2 [101]$                     | $a/2 [\bar{1}\bar{1}0]$         | $a [11\bar{1}]$                                                  | $a/6 [112]$                    | $a/6 [\bar{1}2\bar{1}]$        | $a/3 [11\bar{1}]$                                                 |
| $\Sigma 39$     | $32.204^\circ$ | $a/2 [4\bar{1}3]$               | $a/2 [134]$                     | $a [11\bar{1}]$                                                  | $a/78 [\bar{2}75]$             | $a/78 [752]$                   | $a/3 [11\bar{1}]$                                                 |
| $\Sigma 13$     | $27.796^\circ$ | $a/2 [\bar{4}1\bar{3}]$         | $a/2 [134]$                     | $a/3 [11\bar{1}] + a/6 [\bar{5}27]$<br>$= a/2 [\bar{1}0\bar{3}]$ | $a/26 [\bar{4}1\bar{3}]$       | $a/26 [134]$                   | $a/3 [11\bar{1}] + a/78 [\bar{5}27]$<br>$= a/26 [7\ 8\ \bar{1}1]$ |
| $120.000^\circ$ |                |                                 |                                 |                                                                  |                                |                                |                                                                   |

|               | $\hat{B}_1$<br>(Å) | $\hat{B}_2$<br>(Å) | $\hat{B}_3$<br>(Å) | $[V]$<br>(Å) | $\hat{C}_y^{\text{rot}}$<br>(Å) | $\hat{C}_z^{\text{rot}}$<br>(Å) |
|---------------|--------------------|--------------------|--------------------|--------------|---------------------------------|---------------------------------|
| $\Sigma 3^+$  | +1.035             | 0.000              | 0.825              | 0.086        | -0.657                          | +0.632                          |
| $\Sigma 3^-$  | -1.035             | 0.000              | 0.825              | 0.086        | -0.657                          | +0.632                          |
| $\Sigma 39^+$ | +0.248             | +0.027             | 0.003              | 0.324        | +0.027                          | +0.327                          |
| $\Sigma 39^-$ | -0.248             | -0.027             | 0.003              | 0.324        | -0.027                          | +0.327                          |
| $\Sigma 13^+$ | +0.043             | +0.035             | 0.393              | 0.325        | +0.389                          | +0.605                          |
| $\Sigma 13^-$ | -0.043             | -0.035             | 0.393              | 0.325        | +0.329                          | +0.640                          |

**Supplemental Table S-II:** Microscopic DOFs of GB phases. We found that for each GB phase, two degenerate variants with opposite excess shears exist, indicated by plus or minus, based on the sign of  $\hat{B}_1$ . The values  $\hat{B}_{1,2,3}$  are expressed in the  $xyz$  coordinate system of the GB, as in Figs. 2–4 in the main text. Note that  $C_{1,2} = B_{1,2}$  and  $C_3 = B_3 + [V]$ . The rotated values  $\hat{C}_{y,z}^{\text{rot}}$  correspond to the triple junction's coordinate system (Fig. 1 in the main text). It is  $\hat{C}_x^{\text{rot}} = \hat{B}_1$  (rotation axis).
